# Supplementary material for: A Dynamic Strategy Coach for Effective Negotiation
Source: arXiv:1909.13426 source file (2019-09-30)
Supplement: Supplementary file 1 [file supp.tex]

\documentclass[11pt,a4paper]{article}
\usepackage[hyperref]{acl2019}
\usepackage{times}
\usepackage{latexsym}
\usepackage{url}
\usepackage{xspace}
\usepackage{tabularx}

\usepackage{amsmath}
\usepackage{graphicx}
\usepackage{float}
\usepackage{makecell}
\usepackage{algorithm}
\usepackage{multirow}
\usepackage{booktabs}
\usepackage{textcomp}
\usepackage{bbold}
\usepackage{bibentry} 
\usepackage[noend]{algpseudocode}
\makeatletter
\def\BState{\State\hskip-\ALG@thistlm}
\makeatother
\usepackage{color}

\newcommand{\ignore}[1]{}

\newcommand{\st}[1]{$\langle \textsl{#1} \rangle$}
\newcommand{\ut}[1]{``\textit{#1}''}

\newcommand\possesivecite[1]{\citeauthor{#1}'s (\citeyear{#1})}
 
%% Table
\newcolumntype{L}[1]{>{\raggedright\let\newline\\\arraybackslash\hspace{0pt}}m{#1}}
\newcolumntype{C}[1]{>{\centering\let\newline\\\arraybackslash\hspace{0pt}}m{#1}}
\newcolumntype{R}[1]{>{\raggedleft\let\newline\\\arraybackslash\hspace{0pt}}m{#1}}

%\aclfinalcopy % Uncomment this line for the final submission
%\def\aclpaperid{***} %  Enter the acl Paper ID here

%\setlength\titlebox{5cm}
% You can expand the titlebox if you need extra space
% to show all the authors. Please do not make the titlebox
% smaller than 5cm (the original size); we will check this
% in the camera-ready version and ask you to change it back.

\title{Supplementary Material for \\ A Dynamic Strategy Coach for Effective Negotiation}

\author{First Author \\
  Affiliation / Address line 1 \\
  Affiliation / Address line 2 \\
  Affiliation / Address line 3 \\
  \texttt{email@domain} \\\And
  Second Author \\
  Affiliation / Address line 1 \\
  Affiliation / Address line 2 \\
  Affiliation / Address line 3 \\
  \texttt{email@domain} \\}

\date{}

\begin{document}
\maketitle
\section{Appendices}
\label{sec:appendix}
\subsection{Negotiation Strategies with pattern matching}
\label{sec:strat_pattern_matching}
\begin{itemize}
\item \st{Do not propose first}\\ Waiting for the buyer's proposal allows the seller to
better estimate 
the buyer's target. The detector simply keeps track of who proposes a price first by detecting \st{propose a price}. 
%%%%%%%%%%%%%%%%%%%%%%%%%%%%%
\item \st{Negotiate side offers}\\
The seller sometimes negotiates side offers, e.g., 
throwing in a free gift card or offering free delivery. 
To detect this strategy, we match the turn against a set of phrases, 
e.g., \ut{throw in}, \ut{throwing in}, \ut{deliver}, 
\ut{delivery}, \ut{pick up}, \ut{pick it up}, \ut{in cash}.

\item \st{Use factive verbs} \\defined in \cite{Joan:75} (e.g. \textit{know});
\item \st{Use hedges} \\defined in \cite{ken:05} (e.g. \textit{could, would});
\item \st{Use certainty words}\\ defined in the LIWC dictionary~\cite{tausczik2010psychological}.

\item \st{Communicate politely} \\
We include several politeness-related negotiation 
strategies that were identified by \citet{Danescu:13} 
as most informative predictors. They include: gratitude, greetings , apology, ``please'' in the beginning of a turn, 
``please'' later on. Keywords matching is used to detect these strategies. 

\item \st{Build rapport}\\
Deepening self-disclosure---e.g., ``My kid really liked this bike, but he outgrew it.''---is one strategy for building rapport. We implemented three strategy detectors to identify self-disclosure. First, we count first-person pronouns \cite{Valerian:87,Adam:01}. 
Second, we count mentions of family members and friends, respectively \cite{wang:16}. 
It is done by matching lexicons from \textit{family} and \textit{friend} categories in LIWC.

\item \st{Talk informally} \\ It is detected by matching 
the keywords in the \textit{informal language} category in LIWC. 

\item \st{Show dominance} \\ To detect stubbornness \cite{Chenhao:16}, we measure the average dominance score of all the words from the \possesivecite{Amy:13}'s dominance ratings of 14,000 words.

\item \st{Express negative sentiment}\\ %When, for example, the buyer makes unreasonable proposals, the seller should express negative sentiment to show unwillingness. To identify this strategy, 
We measure both positive and negative sentiments 
by counting words from \textit{positive} and \textit{negative} categories in LIWC.
\end{itemize}

\input{examples.tex}

\newpage
\bibliography{acl2019}
\bibliographystyle{acl_natbib}
\end{document}
